# Supplementary material for: Value of Information in Bayesian Routing Games
Source: arXiv:1808.10590 source file (2020-03-06)
Supplement: Supplementary file 1 [file appendix_social_proof.tex]

%Folowing \cite{roughgarden2004bounding}, we define the Pigou bound $\pg$ as:
%\begin{equation}\label{def_pigou}
%\pg=\sup_{c \in \cfunset} \sup_{x \geq 0, y \geq 0} \frac{y \cdot c(y)}{x \cdot c(x)+(y-x) \cdot c(y)},
%\end{equation}
%where $\cfunset$ is the set of edge cost functions $\{\cesfun(\we)\}_{\e \in \E, \s \in \S}$. We find that the inefficiency in equilibrium is upper bounded by $\pg$. 
%\begin{proposition}\label{pigou_bound}
%For any given $\lamb$, we have $\frac{\clamb}{\copt} \leq \pg$, and the bound is tight. If the edge cost functions $\cesfun(\we)$ are affine functions for all $\e \in \E, \s \in \S$, we have $\frac{\clamb}{\copt} \leq \frac{4}{3}$.
%\end{proposition}
%
%\proof{Proof of Proposition \ref{pigou_bound}.}
%From the definition of BWE in \eqref{eq:BWE_fun}, we obtain:
%\begin{align}
%\sum_{\r \in \R} \qwetir \ecrtiwe=\lambi \D \cdot \min_{\r \in \R} \ecrtiwe \leq \sum_{\r \in \R}  \q^{opt i}_\r(\ti) \ecrtiwe, \quad \forall \ti \in \Ti, \forall \i \in \I.  \label{popu_variation}
%\end{align}
%Define $\l^{opt}$ as the route flow vector induced by an optimal average cost strategy $q^{opt}$, and $\w^{opt}$ as the induced edge load vector. Following \eqref{popu_variation}, we have:
%\begin{align}
%&\sum_{\s \in \S} \sum_{\e \in \E} \sum_{\t \in \T} \pi(\s, \t) \wewe(\t) \cesfun(\wewe(\t))\stackrel[\eqref{eq:ecrti}]{\eqref{eq:q_w}}{=}
%\sum_{\i \in \I} \sum_{\ti \in \Ti} \pro(\ti) \(\sum_{\r \in \R} \qwetir \ecrtiwe\) \notag\\
%\stackrel{\text{\eqref{popu_variation}}}{\leq}& \sum_{\i \in \I} \sum_{\ti \in \Ti} \pro(\ti) \(\sum_{\r \in \R} \qopttir \ecrtiwe\)
%\stackrel[\eqref{eq:ecrti}]{\eqref{eq:q_w}}{=}\sum_{\s \in \S} \sum_{\e \in \E} \sum_{\t \in \T} \pi(\s, \t) \weopt(\t) \cesfun(\wewe(\t)).\label{ineq_variation}
%\end{align}
%This leads to:
%\begin{equation*}
%\begin{split}
%&\copt=\sum_{\s \in \S} \sum_{\e \in \E} \sum_{\t \in \T} \pi(\s, \t) \cesfun\(\weopt(\t)\)\weopt(\t)\\
%=& \sum_{\s \in \S} \sum_{\e \in \E} \sum_{\t \in \T} \pi(\s, \t) \left[\cesfun\(\wewe(\t)\)\wewe(\t) \cdot \frac{\weopt(\t)\cesfun\(\weopt(\t)\) + \(\wewe(\t)-\weopt(\t)\)\cesfun\(\wewe(\t)\)}{\cesfun\(\wewe(\t)\)\wewe(\t) }\right]\\
% +& \sum_{\s \in \S} \sum_{\e \in \E} \sum_{\t \in \T} \pi(\s, \t) \(\weopt(\t)-\wewe(\t)\)\cesfun\(\wewe(\t)\)\\
% \stackrel{\text{\eqref{ineq_variation}}}{\geq}& \(\sum_{\s \in \S} \sum_{\e \in \E} \sum_{\t \in \T} \pi(\s, \t) \cesfun(\wewe(\t))\wewe(\t)\) \cdot \left[\min_{\s \in \S, \e \in \E, \t \in \T} \frac{\weopt(\t)\cesfun\(\weopt(\t)\) + \(\wewe(\t)-\weopt(\t)\)\cesfun\(\wewe(\t)\)}{\cesfun\(\wewe(\t)\)\wewe(\t) }\right]\\
%  \stackrel{\text{\eqref{def_pigou}}}{\geq}&\frac{\clamb}{\pg}.
%\end{split}
%\end{equation*}
%Thus, $\frac{\clamb}{\copt} \leq \pg$. Consider affine cost functions, for any $\e \in \E$ and $\s \in \S$, assuming $\cesfun(\we)=\aes \we+\bes$, we have:
%\begin{align}\label{quater}
%\weopt(\t)\(\cesfun\(\wewe(\t)\)-\cesfun\(\weopt(\t)\)\)=\aes \weopt(\t) \(\wewe(\t)-\weopt(\t)\) \leq \frac{1}{4} \aes \wewe(t)^2 \notag\leq \frac{1}{4} \wewe(\t) \cesfun\(\wewe(\t)\).
%\end{align}
%Thus, we obtain:
%\begin{equation*}
%\begin{split}
%\clamb &=\sum_{\s \in \S} \sum_{\e \in \E} \sum_{\t \in \T} \pi(\s, \t) \wewe(\t) \cesfun(\wewe(\t))  \stackrel{\text{\eqref{ineq_variation}}}{\leq} \sum_{\s \in \S} \sum_{\e \in \E} \sum_{\t \in \T} \pi(\s, \t) \weopt(\t) \cesfun(\wewe(\t))\\
%&= \sum_{\s \in \S} \sum_{\e \in \E} \sum_{\t \in \T} \pi(\s, \t) \weopt(\t) \cesfun(\weopt(\t))+\sum_{\s \in \S} \sum_{\e \in \E} \sum_{\t \in \T} \pi(\s, \t) \weopt(\t) \(\cesfun(\wewe(\t))-\cesfun(\weopt(\t))\)\\
%& \stackrel{}{\leq} \sum_{\s \in \S} \sum_{\e \in \E} \sum_{\t \in \T} \pi(\s, \t) \weopt(\t) \cesfun(\weopt(\t))+	\frac{1}{4} \sum_{\s \in \S} \sum_{\e \in \E} \sum_{\t \in \T} \pi(\s, \t) \wewe(\t) \cesfun(\wewe(\t))\\
%&=\copt+\frac {1}{4} \clamb.
%\end{split}
%\end{equation*}
%Therefore, $\frac{\clamb}{\copt} \leq \frac{4}{3}$. Since the game with one population, one state is a special case of our game, and the bound $\kappa(\cfunset)$ is tight, we can conclude that the bound is tight as well in $\game$.  \Halmos
%\endproof
%
%The social optimal cost $\cso$ is defined as follows:
%\begin{equation}\label{cso_def}
%\begin{split}
%C^{so} \deleq &\min_{\l} \sum_{\s \in \S} \sum_{\e \in \E} c_\e^\s(\sum_{\r \ni \e} \l_\r^\s),\\
%s.t. \quad & \sum_{\r \in \R}\l_\r^\s=\D, \quad \forall \s \in \S, \\
%& \l_r^\s \geq 0, \quad \forall \r \in \r, \quad \forall \s \in \S,
%\end{split} 
%\end{equation}
%
%\proof{Proof of Proposition \ref{homo_bathtub}.}
%We first show that $\frac{\clamb}{\copt}=1$. For any feasible strategy profile $\q \in \Q$, $C(\q)$ can be written as:
%\begin{align*}
%C(\q)&=\frac{1}{\D} \sum_{\i \in \I}\sum_{\ti \in \Ti} \pro(\ti) \sum_{\r \in \R} \ecrti \qtir\stackrel[\eqref{eq:ecrti}]{\eqref{eq:q_w}}{=}\frac{1}{\D} \sum_{\s \in \S} \sum_{\e \in \E} \sum_{\t \in \T}\pi(\s, \t)\cesfun\(\we(\t)\)\cdot \we(\t)\\
%&\stackrel{\eqref{eq:q_w}}{=}\frac{1}{\D} \sum_{\s \in \S} \sum_{\e \in \E} \sum_{\t \in \T}\pi(\s, \t) \int_{0}^{\sum_{\r \ni \e} \sum_{\i \in \I} \qtir} \frac{d \(\cesfun(x) \cdot x\) }{d x} d x\\
%&=\frac{1}{\D} \sum_{\s \in \S} \sum_{\e \in \E} \sum_{\t \in \T}\pi(\s, \t) \int_{0}^{\sum_{\r \ni \e} \sum_{\i \in \I} \qtir}\(\cesfun(x)+x \cdot \frac{d \cesfun(x)}{d x}\)dx.
%\end{align*}
%Assume that the condition of the edge cost functions in Proposition \ref{homo_bathtub} is satisfied. Since $h_e^s(\cdot)$ is a k-th order homogeneous function of $\we$, we know from Euler's homogeneous function theorem that $x \cdot \frac{d h_e^s(x)}{dx}=k \cdot h_e^s(x)$. Therefore, $\cesfun(x)+x \cdot \frac{d \cesfun(x)}{d x}= h_e^s(x)+\f_e^s+x \cdot \frac{\partial h_e^s(x)}{\partial x}=(k+1) \cdot h_e^s(x)+\f_e^s$. The cost $C(\q)$ can be further expressed as:
%\begin{align}
%C(\q)&=\frac{1}{\D}\sum_{\e \in \E} \sum_{\t \in \T} \sum_{\s \in \S} \pi(\s, \t) \int_{0}^{\sum_{\r \ni \e} \sum_{\i \in \I} \qtir} (k+1) \cdot h_e^s(x) dx +\frac{1}{\D} \sum_{\e \in \E} \sum_{\t \in \T} \sum_{\s \in \S} \pi(\s, \t) \int_{0}^{\sum_{\r \ni \e} \sum_{\i \in \I} \qtir} \f_\e^{\s} dx  \notag\\
%&=\frac{k+1}{\D}\sum_{\e \in \E} \sum_{\t \in \T} \sum_{\s \in \S} \pi(\s, \t) \int_{0}^{\sum_{\r \ni \e} \sum_{\i \in \I} \qtir} \(h_e^s(x)+\f_\e^\s\) dx -\frac{k}{\D} \sum_{\e \in \E} \sum_{\t \in \T} \sum_{\s \in \S} \pi(\s, \t) \int_{0}^{\sum_{\r \ni \e} \sum_{\i \in \I} \qtir} \f_\e^{\s} dx  \notag\\
%&\stackrel{\eqref{eq:q_w}}{=}\frac{k+1}{\D}\sum_{\e \in \E} \sum_{\t \in \T} \sum_{\s \in \S} \pi(\s, \t) \int_{0}^{\sum_{\r \ni \e} \sum_{\i \in \I} \qtir} \cesfun(x) dx - \frac{k}{\D} \sum_{\e \in \E} \sum_{\t \in \T} \sum_{\s \in \S} \pi(\s, \t)  \f_\e^{\s}\we(\t)  \notag\\
%&\stackrel{\eqref{eq:potential_q}}{=}\frac{(k+1)}{\D}\potential(\q)-\frac{k}{\D} \sum_{\s \in \S} \sum_{\t \in \T} \pi(\s, \t) \cdot \(\sum_{\r \in \R} \(\sum_{\e \in \r} \f_\e^\s\) \cdot \lr(\t)\)\notag
%\end{align}
%Moreover, since $\sum_{\e \in \r} b_e^s =b^\s$ for any $\s \in \S$, and any $\r \in \R$, we obtain:
%\begin{align}
%C(\q)&= \frac{(k+1)}{\D}\potential(\q)-\frac{k}{\D} \sum_{\s \in \S} \sum_{\t \in \T} \pi(\s, \t) \cdot \(\sum_{\r \in \R} b^\s \cdot \lr(\t)\)\notag\\
%&\stackrel{\eqref{sub:ldemand}}{=}\frac{(k+1)}{\D}\potential(\q)-k \cdot  \(\sum_{\s \in \S} \(\sum_{\t \in \T} \pi(\s, \t)\) \cdot \f^s\) =\frac{(k+1)}{\D}\potential(\q)-k \cdot  \(\sum_{\s \in \S} \ps(\s) \cdot \f^s\)\label{final_step}.
%\end{align}
%Since the equilibrium strategy profile $\qwe$ minimizes $\potential(\q)$, $\qwe$ also minimizes $C(\q)$. Thus, $\frac{\clamb}{\copt}=1$. 
%
%Additionally, from \eqref{final_step}, we obtain that: 
%\begin{align*}
%\clamb=\copt=\min_{\q \in \Q(\lamb)} C(\q)\stackrel{\eqref{final_step}}{=}\frac{(k+1)}{\D}\Plamb-k \cdot  \(\sum_{\s \in \S} \ps(\s) \cdot \f^s\).
%\end{align*}
%Therefore, $\clamb$ is an affine function of $\Plamb$. From Lemma \ref{lemma_minimum_lambdag}, we know that $\Lambdag=\argmin_{\lamb \in \Lamb} \Plamb$. Consequently, $\Lambdag=\argmin_{\lamb \in \Lamb} \clamb$. \Halmos
%\endproof
